# Supplementary material for: HalluCounter: Reference-free LLM Hallucination Detection in the Wild!
Source: arXiv:2503.04615 source file (2025-05-27)
Supplement: Supplementary file 1 [file kaggle_confidence_scores.tex]

\begin{table*}
\resizebox{\textwidth}{!}{
\begin{tabular}{c|c|c|c|c|c|c|c}
\hline
Category                     & ENSB-Gen & GM-7B-Gen & LL-70B-Gen & LL-8B-Gen  & MST-7B-Gen & PHI-3.5B-Gen & TL-1.1B-Gen \\ \hline
GK       & 93       & 98        & 93                 & 96         & 89      & 96   & 85        \\ \hline
MathQA   & 96       & 92        & 94                 & 90         & 96      & 95   & 100       \\ \hline
MathQSA  & 93       & 96        & 92                 & 89         & 91      & 87   & 98        \\ \hline
SciQ     & 91       & 93        & 89                 & 96         & 87      & 97   & 80        \\ \hline
\end{tabular}
}
\caption{Confidence Score for each category in Kaggle dataset across various test sets generated by LLMs}
\label{tab:kaggle_confidence_scores}
\end{table*}
