# Supplementary material for: HalluCounter: Reference-free LLM Hallucination Detection in the Wild!
Source: arXiv:2503.04615 source file (2025-05-27)
Supplement: Supplementary file 2 [file kaggle_hallucination_rates.tex]

\begin{table*}
\resizebox{\textwidth}{!}{
\begin{tabular}{c|c|c|c|c|c|c|c}
\hline
Category                     & ENSB-Gen & GM-7B-Gen & LL-70B-Gen & LL-8B-Gen  & MST-7B-Gen & PHI-3.5B-Gen & TL-1.1B-Gen \\ \hline
GK       & 0        & 0         & 0                  & 0          & 0       & 0    & 1         \\ \hline
MathQA   & 61       & 52        & 55                 & 55         & 59      & 58   & 65        \\ \hline
MathQSA  & 8        & 8         & 8                  & 7          & 8       & 7    & 10        \\ \hline
SciQ     & 3        & 11        & 3                  & 0          & 8       & 0    & 11        \\ \hline
\end{tabular}
}
\caption{Hallucination Rate for each category in Kaggle dataset across various test sets generated by LLMs}
\label{tab:kaggle_hallucination_rates}
\end{table*}
